# Supplementary material for: Stable solid molecular hydrogen above 900K from a machine-learned potential trained with diffusion Quantum Monte Carlo
Source: arXiv:2209.00658 source file (2023-02-15)
Supplement: Supplementary file 1 [file supplemental.tex]

\section{Supplementary Material}\label{supplemental}
\subsection{Data generation}
We have generated training data with QMC forces and made them publicly available on yt Hub\cite{ythub}. We included many hydrogen configuration snapshots obtained from classical MD, path integral molecular dynamics (PIMD), and coupled electron-ionic Monte Carlo (CEIMC) simulations. In Fig.~\ref{fig:data-grid} we show the grid of temperatures and pressures where our simulations were performed. From approximately 100,000 configurations each with 96 protons, the total energy and the forces on each atom of a configuration are evaluated with DFT using both PBE and vdW-DF1 functionals. A subset of approximately 20,000 configurations was used for diffusion Monte Carlo (DMC) calculations as described below, to obtain accurate forces providing a large database for training machine-learned interatomic potentials for hydrogen. 
\begin{figure}[tbh]
\centering
\includegraphics[width=1.01\linewidth]{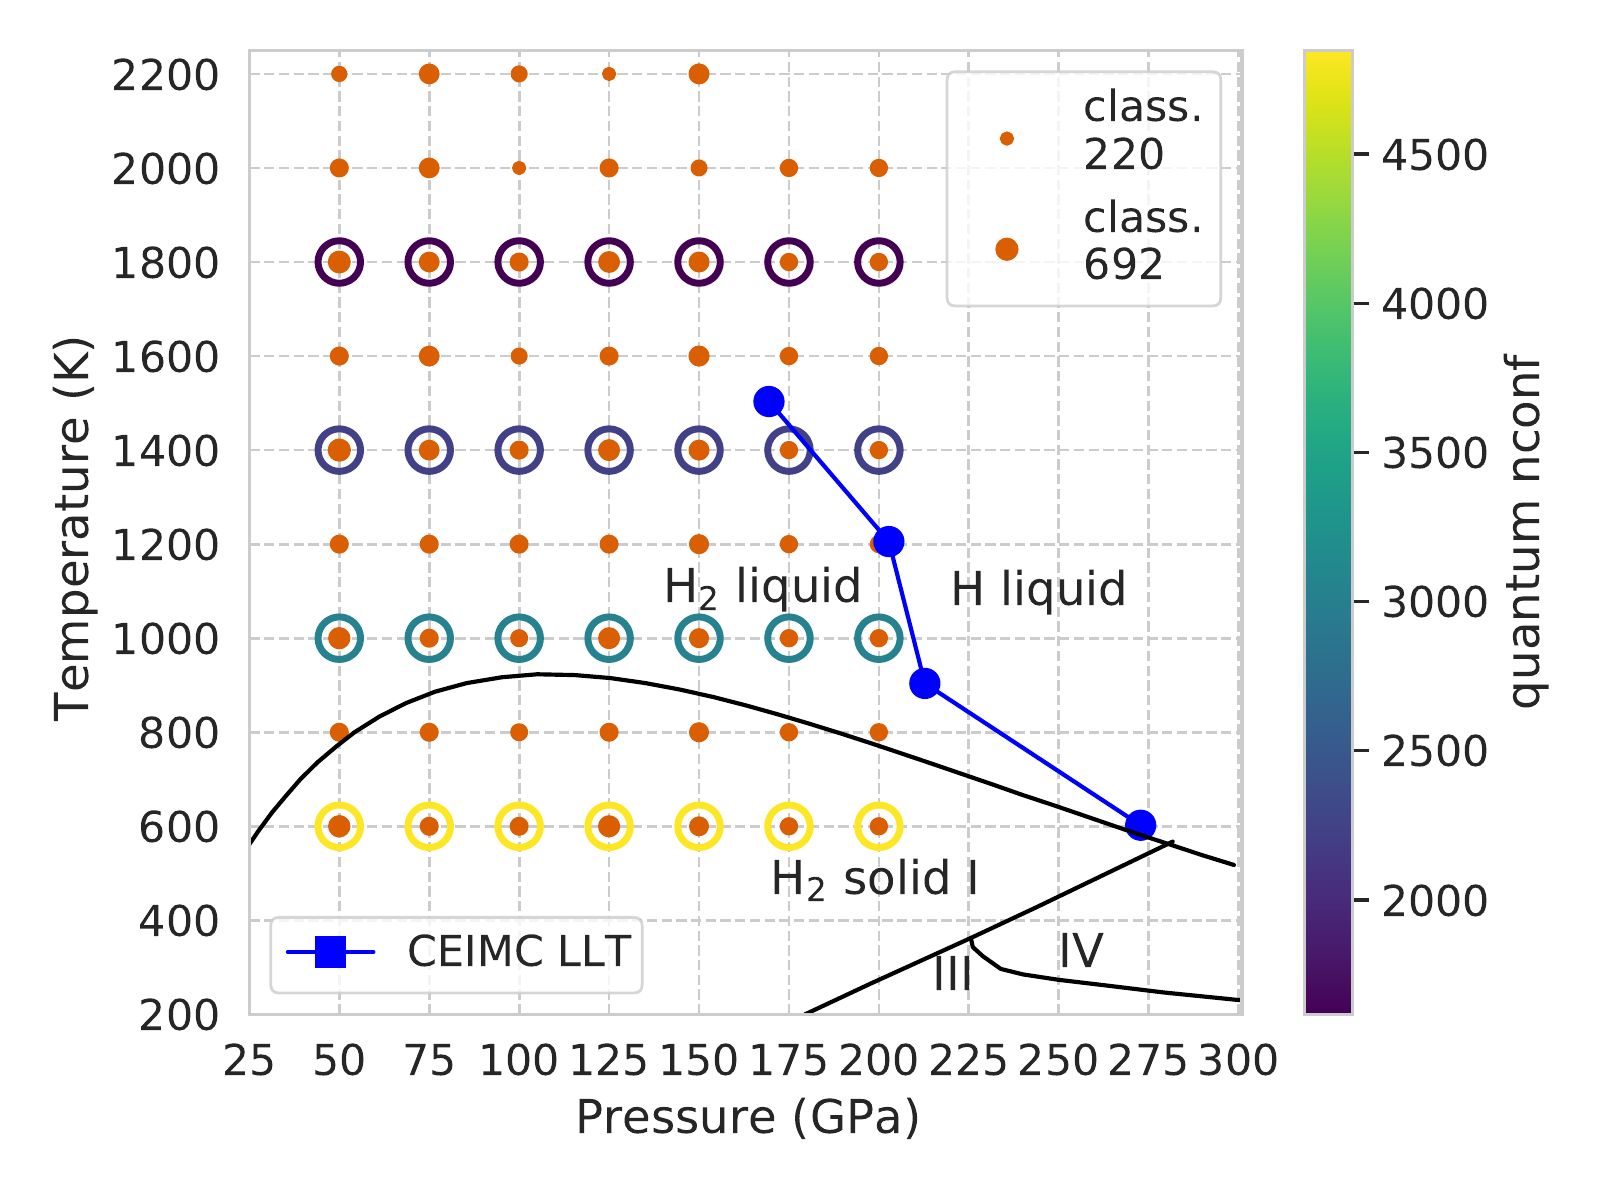}
\caption{Hydrogen data selection. The grid points indicate where simulations were performed. This is overlaid on the phase diagram for hydrogen of Ref.~\cite{RMP2012}. Larger grid points represent larger number of classical proton configurations (692) and smaller points show pressures and temperatures with less configurations (220). The circles around these grid points show the number of quantum proton configurations in our database indicated with the colorbar.}
\label{fig:data-grid}
\label{fig:hydrogen_data}
\end{figure}

\subsubsection{DFT calculations}
%https://girder.hub.yt/#item/5f777c6468085e0001d27b77
We used Quantum Espresso (QE)\cite{Giannozzi2009,Enkovaara2017} version 6.5 and 6.7 for all DFT calculations. 
DFT energy, forces, and stresses were calculated using a norm-conserving pseudopotential \verb|H.pbe-rrkjus_psl.1.0.0.UPF|, a planewave cutoff of 96 Ry on a $4\times4\times4$ shifted k-grid. Occupations of the Kohn-Sham orbitals are smeared by the Fermi-Dirac function at $1000$ K.

\subsubsection{DMC calculations}
%https://girder.hub.yt/#item/6034089268085e0001d2aaf1
The FN-DMC calculations were done with QMCPACK version 3.9.2~\cite{Kim2018,Kent2020}. They used a Slater-Jastrow trial wavefunction. The Slater determinant consisted of PBE orbitals using a Troullier-Martins PBE pseudopotential, with core radius $r_c=0.37 a_0$ ($a_0$ indicates the Bohr radius), and a planewave cutoff $200$ Ry.
The Jastrow functions contain two-body correlations as a sum of short-range (represented by Bsplines) and long-range contributions both
fully optimized for each configuration.

The FN-DMC calculations used $>2000$ walkers and projected for $100$ ha$^{-1}$ at a timestep of $0.02$ ha$^{-1}$.
Canonical twist-averaging was performed on a $4\times4\times4$ shifted twist grid.
We used the Chiesa force estimator \cite{Chiesa2005} with fitting radius $\mathcal{R}=1.0~a_0$, basis size $M=4$ and a weighting exponent of $m=2$.
Mixed-estimator bias on the forces were corrected using the linear extrapolation formula $2*DMC-VMC$.
Finite-size corrections were applied to the total energy~\cite{Chiesa2006,Holzmann2016} using the computed structure factor.

\subsection{Model Training}
%\begin{figure*}[tbh]
%\includegraphics[width=0.7\linewidth]{final_model}
%\caption{Detailed workflow to build the DMC trained ML model in a hierarchical way}
%\label{fig:final-model}
%\end{figure*}
%\SJ{Commented out workflow diagram; describe full workflow in words, see if diagram is useful and assists in description.}

The DMC trained ML model adopt a hierarchical approach: it is a sum of three terms (see eq.~(1) in the main text). % and the detailed workflow to build each term is shown in figure~\ref{fig:final-model}.
%Based on the DMC data set, we trained a machine learning (ML) potential to study the phase diagram of dense hydrogen. 
The Deep Potential Molecular Dynamics (DPMD)~\cite{Han2018,Zhang2018a,Zhang2018} framework is employed and the cutoff radius $R_c$ of the ML potential is first determined by a ``locality test''~\cite{Bartok2010}. %$R_c$ of the local atomic environment is a very important parameter of the ML model.
If the force on one single atom depends on environment outside of $R_c$, then errors will be introduced when calculating the forces on the atom with ML model.
%To obtain the minimum cutoff radius to describe the dense hydrogen atomic environment, the ``locality test'' is performed.
As shown in Fig.~\ref{fig:locality-test},
\begin{figure}[h]
\includegraphics[width=\columnwidth]{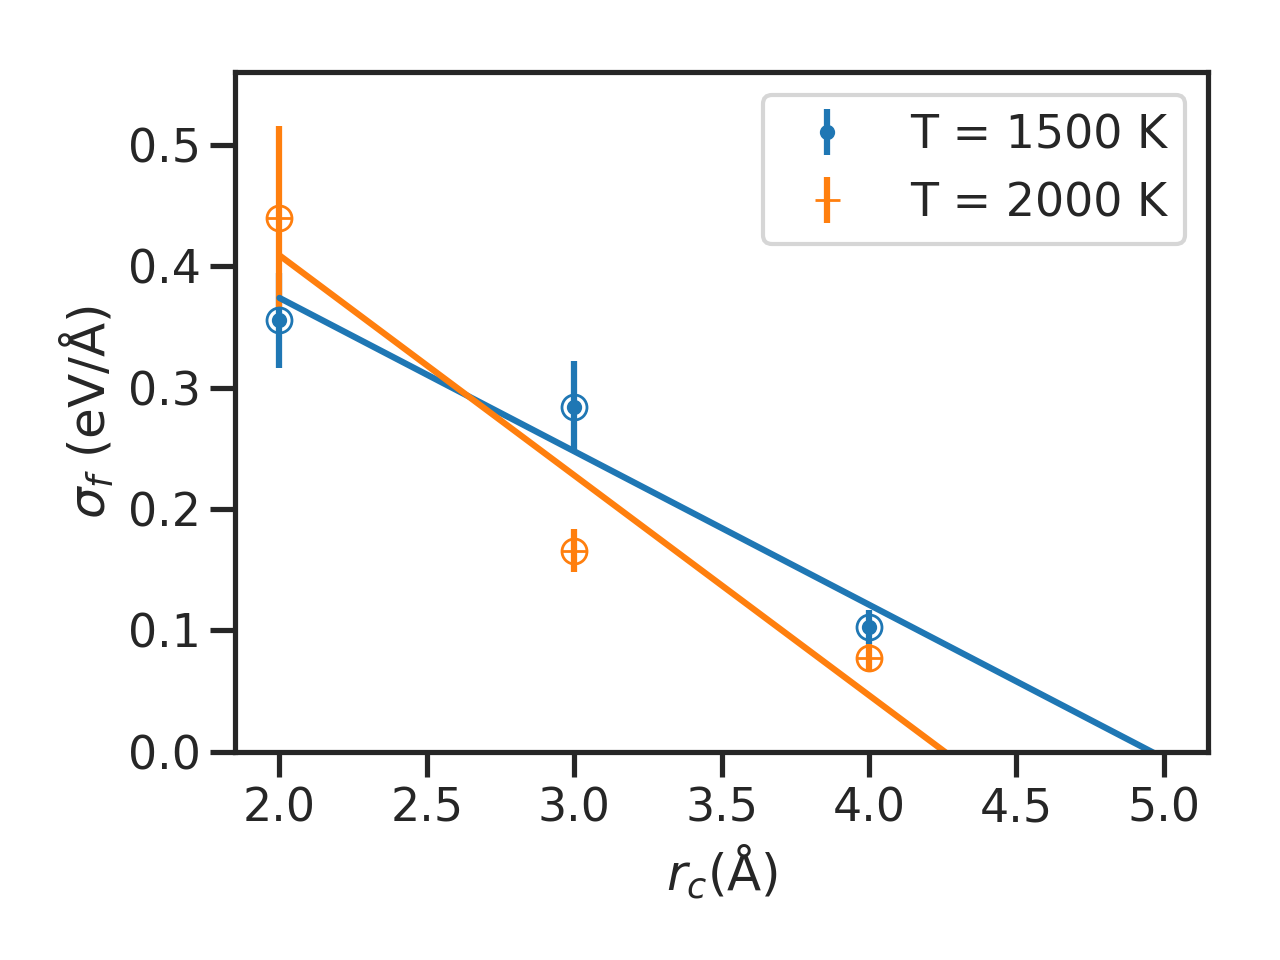}
\caption{Locality test: variance of force on central atom in MD as a function of the cutoff radius.}
\label{fig:locality-test}
\end{figure}
we fixed the atoms inside the cutoff radius of one single atom and performed MD simulations at 1500 K and 2000 K to change the positions of the atoms outside the cutoff radius, and then calculated the forces on the single atom using DFT.
%We found that the force variance decreased as the cutoff radius increased. 
Cutoff radii larger than 5.0 \AA~ are enough to describe the dense hydrogen atomic environment.

We use DeePMD version 1.3.3 to train the the ML models.
Symmetry invariant feature vectors for atomic environments are constructed via the ``smooth edition''~\cite{Zhang2018} descriptors with angular and radial information (``se\_ar'').
The angular features are smoothly cut off from $3.4$ to $4.0$~\AA, and radial features from $5.1$ to $6.0$~\AA.
We use $8$ neurons in the embedding layer, and $3$ layers of $8$ hidden neurons each for the descriptor network.
The fitting network consists of $4$ layers of $16$ neurons each.

The training process contains $10^6$ iterations. $8$ configurations, each containing $96$ atoms, are used to update the neural network parameters at each iteration. The starting and ending learning rates are set to $5\times 10^{-3}$ and $2\times 10^{-7}$, respectively. The learning rate decreases exponentially during the training process. %A deep neural network of four hidden layers each having 16 nodes was employed to map the local atomic environment to the atomic energy contributions.
% Ricky reply to carlo: "each time" means "each iteration". "each time" is David's style

%test error of DMC trained model
The internal statistical error of each DMC energy per atom is approximately 0.1 meV and 130 meV/\AA~for the forces.  Based on the DMC trained model, the resulting root mean squared error (RMSE) of energy and force over the whole test set was found to be 13.21 meV per atom and 297.3 meV/\AA, respectively.
The RMSE of the energy and forces are defined as
\begin{eqnarray}
E_{RMSE}&=&\sqrt{\frac{1}{M}\sum_{i=1}^M\left(E_i^{\text{Model}}-E_i^{\text{DMC}}\right)^2}, \\
F_{RMSE}&=&\sqrt{\frac{1}{M}\sum_{i=1}^M\frac{1}{3N}\sum_{j=1}^{3N}\left(F_{ij}^{\text{Model}}-F_{ij}^{\text{DMC}}\right)^2},
\end{eqnarray}
where $M$ is the number of test configurations, and $N$ is the number of atoms in each configuration.
$E^{\text{Model}}$ and $F^{\text{Model}}$ are the energy and forces as defined in eq.~(1) in the main text.
The RMSE of the atomic force over the test set as a function of temperature and pressure is shown in Fig.~\ref{fig:test_error}.
% Update of this figure is needed
\begin{figure}[h]
\includegraphics[width=\linewidth]{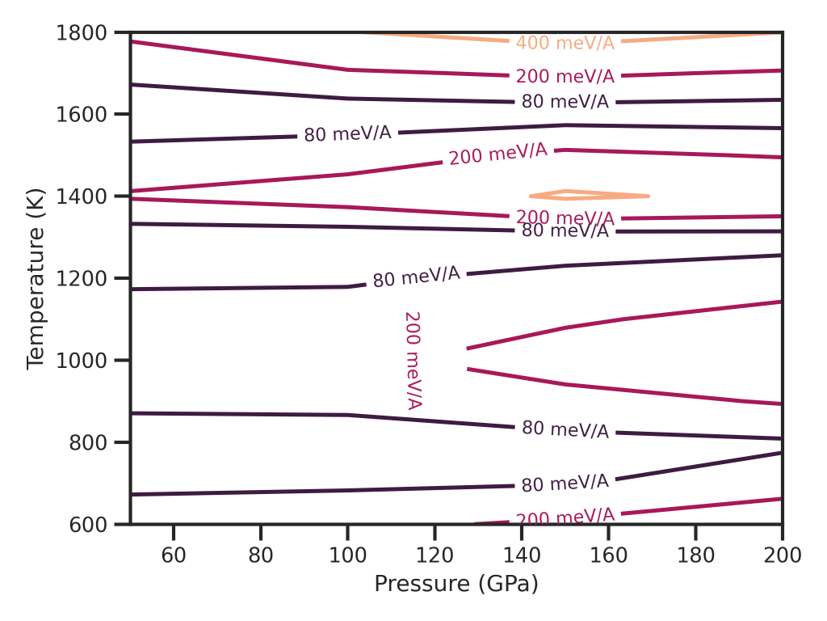}
\caption{Resulting RMSE of force over the test set with DMC trained model}
\label{fig:test_error}
\end{figure}

\subsection{MD Simulations}

All simulations of hydrogen assuming classical proton were carried out using the LAMMPS package~\cite{LAMMPS}. Path integral molecular dynamics (PIMD) simulation for quantum protons were  carried out using the i-Pi Package~\cite{kapil2019pi}.

%\subsubsection{Phase Diagram}
To obtain the phase diagram of dense hydrogen, we performed PIMD simulation over a range of pressures (50 GPa - 225 GPa) and temperatures (50 K - 1600 K) with a grid of 100 K and 25 GPa. Finer grids were used near the experimental I'-III phase boundary. With PIMC $N_b=16$ beads where used for $T>400~K$ while $N_b=48$ beads were used for $T<400~K$.  
The fictitious mass of the beads was taken to be the physical mass of the protons. The timestep was set to 0.1 fs.
All simulations started from a 768-atom system of molecular HCP solid and used an NPT ensemble for $T=5~ps$ to ensure equilibration. The phase diagram was determined using the equilibrated structures, the rotational distributions and the structure factors.

%
%\subsubsection{Molecular Melting}
\begin{table}[h]
 \caption{The results of the two-phase determination of the melting temperature as a function or pressure with DMC-trained model. T$_{\text{solid}}^{\text{q}}$ is the highest temperature with a stable solid of quantum protons. T$_{\text{liquid}}^{\text{q}}$ is the lowest temperature with a stable liquid of quantum protons. T$_{\text{solid}}^{\text{c}}$ is the highest temperature with a stable solid of classical protons. T$_{\text{liquid}}^{\text{c}}$ is the lowest temperature with a stable liquid of classical protons.  
 }
\centering
\begin{tabular}{|c|c|c|c|c|}
\hline
P (GPa) & T$_{\text{solid}}^{\text{q}}$ (K) & T$_{\text{liquid}}^{\text{q}}$ (K) & T$_{\text{solid}}^{\text{cl}}$ (K) & T$_{\text{liquid}}^{\text{cl}}$ (K)\\
\hline
50 & 820 & 860 & 840 & 860 \\
75 & 1040 & 1100 & 1080 & 1090 \\
100 & 1300 & 1320 & 1320 & 1340\\
125 & 1420 & 1440 & 1400 & 1410\\
150 & 1440 & 1460 & 1580 & 1600\\
175 & 1340 & 1360 & 1590 & 1600\\
200 & 1120 & 1140 & 1380 & 1400\\
\hline
\end{tabular}
\label{tab:dmc-melting}
\end{table}

\begin{table}[h]
 \caption{The results of the two-phase determination of the melting temperature as a function or pressure with PBE-trained model.  
 }
\centering
\begin{tabular}{|c|c|c|c|c|}
\hline
P (GPa) & T$_{\text{solid}}^{\text{q}}$ (K) & T$_{\text{liquid}}^{\text{q}}$ (K) & T$_{\text{solid}}^{\text{cl}}$ (K) & T$_{\text{liquid}}^{\text{cl}}$ (K)\\
\hline
50 & 720 & 740 & 740 & 760\\
75 & 860 & 880 & 920 & 930\\
100 & 900 & 920 & 1010 & 1020\\
125 & 800 & 820 & 1020 & 1030\\
150 & 780 & 800 & 1000 & 1020\\
175 & 700 & 720 & 940 & 950\\
200 & 620 & 640 & 880 & 900\\
\hline
\end{tabular}
\label{tab:pbe-melting}
\end{table}

\begin{table}[h]
 \caption{The results of the two-phase determination of the melting temperature as a function or pressure with vdW-DF1-trained model.
 }
\centering
\begin{tabular}{|c|c|c|c|c|}
\hline
P (GPa) & T$_{\text{solid}}^{\text{q}}$ (K) & T$_{\text{liquid}}^{\text{q}}$ (K) & T$_{\text{solid}}^{\text{cl}}$ (K) & T$_{\text{liquid}}^{\text{cl}}$ (K)\\
\hline
50 & 840 & 860 & 840 & 860\\
75 & 960 & 1020 & 1000 & 1020\\
100 & 1100 & 1120 & 1140 & 1160\\
125 & 1100 & 1140 & 1220 & 1240\\
150 & 1120 & 1140 & 1260 & 1280\\
175 & 1080 & 1100 & 1280 & 1300\\
200 & 1040 & 1060 & 1220 & 1240\\
\hline
\end{tabular}
\label{tab:vdw-melting}
\end{table}

To determine the melting temperature of dense hydrogen, we performed PIMD two-phase coexistence simulations with a supercell of $N_p=3,072$ protons over a range of pressures (50 GPa - 200 GPa) in steps of 25 GPa. The PIMD trajectory began with a configuration containing a solid-liquid interface thus eliminating the need to overcome a free energy barrier in transforming between the two phases.
%\david{We also do two-phase for the solid=solid transition, correct? Maybe we should move to methods section?}\ricky{The Solid-solid transition line was calculated from PIMD with NPT ensemble and initial structure of mHCP phase, not from the two-phase approach. The reason why we do not use the two-phase method is when we put the two solid phase together there is always some mismatches that may bias the transition point.}
When ran in an ensemble without a thermostat, e.g. NVE, NPH, the temperature of the two-phase system automatically adjusts to the melting point so long as the interface can be moved sufficiently far into one phase without entirely consuming it. In a path-integral simulation, one must define temperature to define the action. There, we run in the NPT ensemble long enough to allow one phase to dominate the supercell thus bracketing the melting point at a given pressure. Those results, which are upper and lower bounds to the melting temperature are shown in tables I, II and III. The comparison of melting lines from different electronic structure methods are shown in Fig.~8.

\begin{figure}[h]
\includegraphics[width=\linewidth]{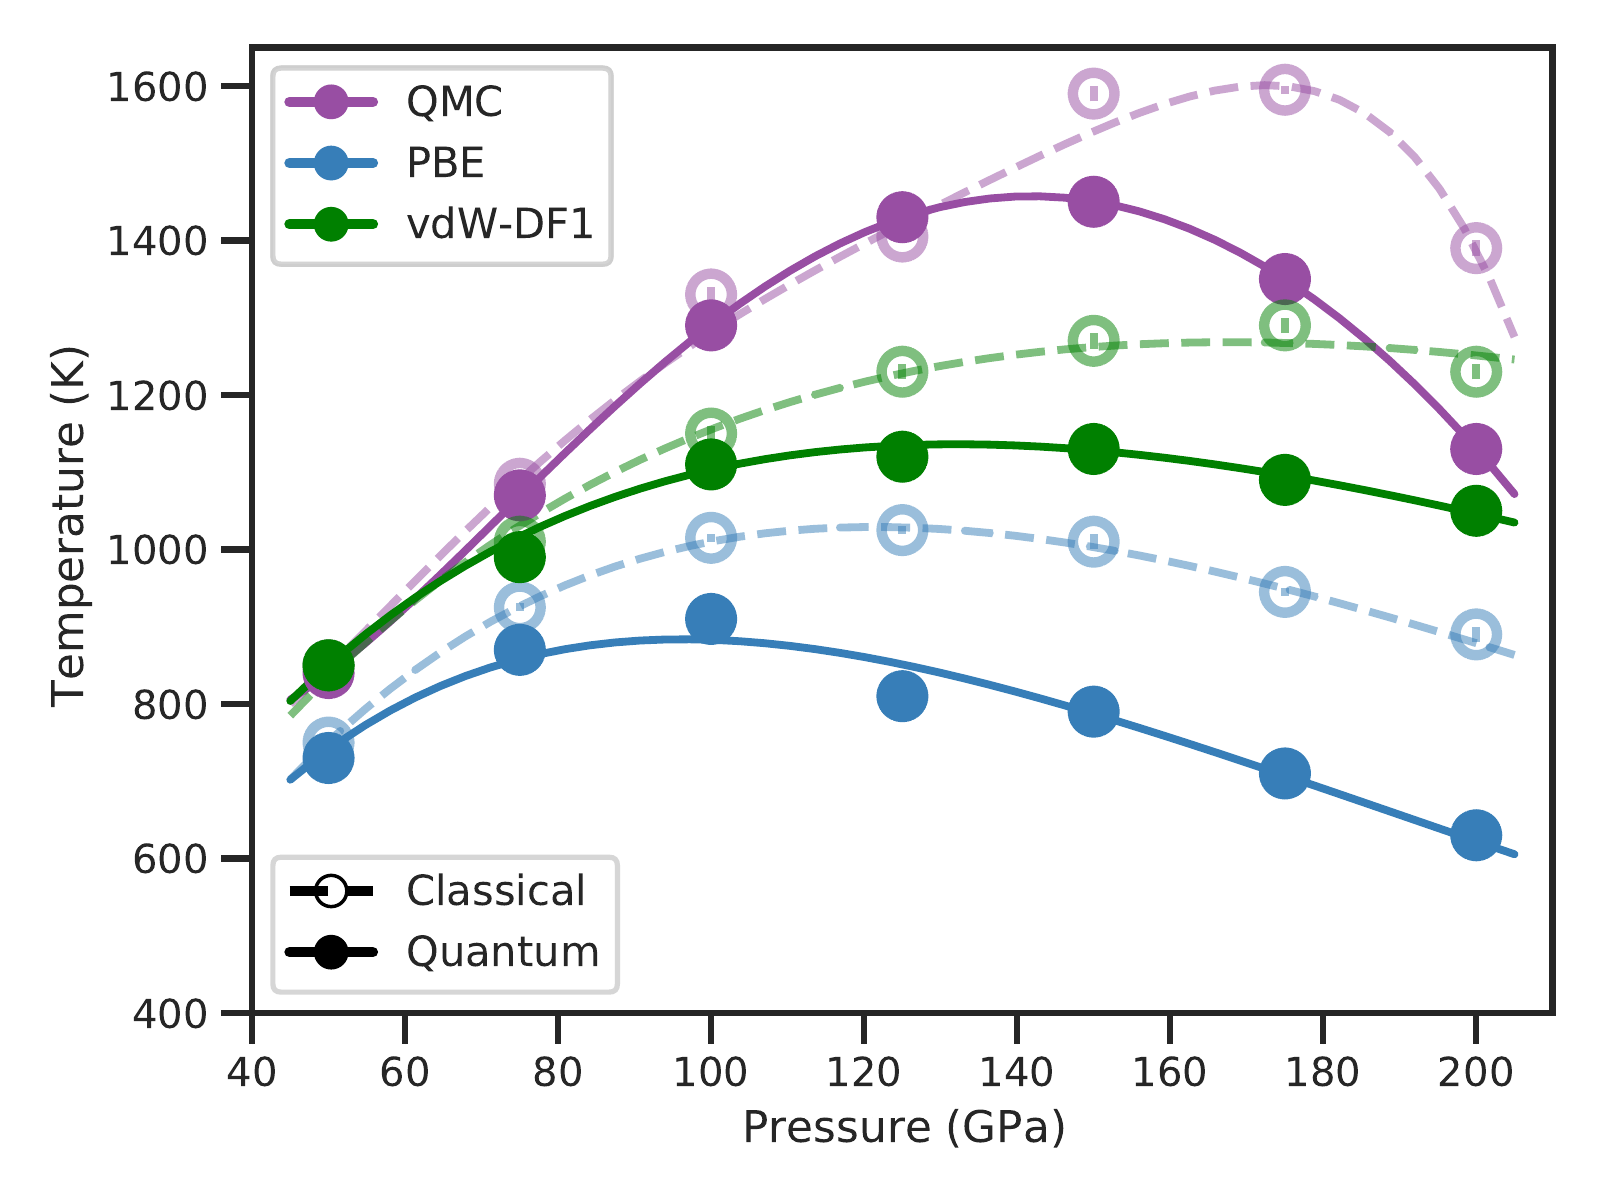}
\caption
{
Comparison of melting lines from various theories. 
Circles are our two-phase results using ML constrained by data from different electronic structure methods. Open symbols represent classical protons, solid symbols quantum protons. The QMC line changes much more rapidly with pressure above the maximum with respect to the DFT lines.
}
\label{fig:ML_melting_compare}
\end{figure}

\subsection{Fmmm-4 crystal structure}

The Fmmm-4 crystal structure has a unit cell that is distorted from that of a HCP lattice. The cell distortion can be parameterized by the $\gamma$ angle, which we find to be approximately $70.5^\circ$ (see panel (a) of Fig. 3 in the main text).  The three primitive vectors of the unit cell are
\begin{eqnarray}
\label{eq:abc}
\bs{a}_1 &=& a~\hat{\bf x} \\ 
\bs{a}_2 &=& 2a\sin(\frac{\gamma}{2}) (\cos(\frac{\pi-\gamma}{2})\hat{\bf x} +  \sin(\frac{\pi-\gamma}{2})\hat{\bf y}) \\
\bs{a}_3&= &c~\hat{\bf z}
\end{eqnarray}

The fractional coordinates of the centers of the two molecules are $(0, 0, 0)$ and $(0, 0.5, 0.5)$. Those of the protons depend on the actual H$_2$ bond length, but they are generally close to the values shown in Table~IV.
\begin{table}[h]
\caption{Fractional coordinates of protons in the ideal oriented Fmmm-4 crystal structure.}
\label{tab:fmmm4-fracs}
\begin{tabular}{lccc}
\toprule
H1 & -0.25 & -0.125 & 0 \\
H2 & 0.25 &  0.125 & 0 \\
H3 & -0.25 &  0.375 & 0.5 \\
H4 & 0.25 &  0.625 & 0.5 \\
\bottomrule
\end{tabular}
\end{table}
